# Supplementary material for: Higher-order organization of complex networks
Source: arXiv:1612.08447 source file (2016-12-26)
Supplement: Supplementary file 1 [file SM-celegans-table.tex]

ADFL & no & Amphid neuron \\
    ADLR & no & Amphid neuron \\
    AFDR & no & Amphid finger cell \\
    AIAL & no & Amphid interneuron \\
    AIAR & no & Amphid interneuron \\
    AIZL & no & Amphid interneuron \\
    AIZR & no & Amphid interneuron \\
    ASER & no & Amphid neurons \\
    ASGL & no & Amphid neurons \\
    ASIL & no & Amphid neurons \\
    ASJL & no & Amphid neurons \\
    ASKL & no & Amphid neurons \\
    AVHL & no & Neuron, mainly postsynaptic in ventral cord and presynaptic in the ring \\
    AVHR & no & Neuron, mainly postsynaptic in ventral cord and presynaptic in the ring \\
    AVJL & no & Neuron, synapses like AVHL/R \\
    AVJR & no & Neuron, synapses like AVHL/R \\
    AWAR & no & Amphid wing cells \\
    AWCR & no & Amphid wing cells \\
    CEPDR & yes & Cephalic neurons \\
    CEPVR & yes & Cephalic neurons \\
    IL1VR & no  & Inner labial neuron \\
    IL2R &  yes & Inner labial neuron \\
    IL2VL & no & Inner labial neuron \\
    IL2VR & no & Inner labial neuron \\
    OLLR & yes & Lateral outer labial neurons \\
    OLQVL & no & Quadrant outer labial neuron \\
    OLQVR & no & Quadrant outer labial neuron \\
    RIAL & yes & Ring interneuron \\
    RIAR & yes & Ring interneuron \\
    RIBR & no & Ring interneuron \\
    RIH & no & Ring interneuron \\
    RIVL & yes &Ring interneuron \\
    RIVR & yes & Ring interneuron \\
    RMDDR & yes & Ring motor neuron/interneuron \\
    RMDL & yes & Ring motor neuron/interneuron \\
    RMDR & yes & Ring motor neuron/interneuron \\
    RMDVL & yes & Ring motor neuron/interneuron \\
    RMFL & yes & Ring motor neuron/interneuron \\
    SMDDL & yes & Ring motor neuron/interneuron \\
    SMDDR & yes & Ring motor neuron/interneuron \\
    SMDVR & yes & Ring motor neuron/interneuron \\
    URBR & yes & Neuron, presynaptic in ring, ending in head \\
